# Supplementary material for: Identification of nuclear effects in neutrino-carbon interactions at low three-momentum transfer
Source: arXiv:1511.05944 source file (2019-09-20)
Supplement: Supplementary file 1 [file appendix.tex]

\setcounter{totalnumber}{5}
\setcounter{bottomnumber}{3}
\setcounter{topnumber}{3}
\setcounter{dbltopnumber}{3}

\onecolumngrid
\appendix{Appendix: Supplementary Material}\hfill\vspace*{4ex}\

\begin{verbatim}
Bin (GeV)  Flux
----------------
2.00-2.10	6.02
2.10-2.20	6.34
2.20-2.30	6.72
2.30-2.40	7.15
2.40-2.50	7.39
2.50-2.60	7.69
2.60-2.70	7.98
2.70-2.80	8.24
2.80-2.90	8.50
2.90-3.00	8.75
3.00-3.10	8.87
3.10-3.20	8.88
3.20-3.30	8.85
3.30-3.40	8.59
3.40-3.50	8.38
3.50-3.60	7.98
3.60-3.70	7.52
3.70-3.80	7.04
3.80-3.90	6.42
3.90-4.00	5.89
4.00-4.10	5.31
4.10-4.20	4.73
4.20-4.30	4.17
4.30-4.40	3.72
4.40-4.50	3.26
4.50-4.60	2.89
4.60-4.70	2.57
4.70-4.80	2.23
4.80-4.90	2.02
4.90-5.00	1.82
5.00-5.10	1.65
5.10-5.20	1.50
5.20-5.30	1.40
5.30-5.40	1.27
5.40-5.50	1.20
5.50-5.60	1.12
5.60-5.70	1.06
5.70-5.80	1.01
5.80-5.90	0.96
5.90-6.00	0.90
\end{verbatim}
\bigskip
Table I:  The $\nu_\mu$ flux, in units 10$^{-5}$ / m$^{2}$ / P.O.T. / GeV

\clearpage
\pagebreak

\begin{verbatim}
                         q3
     =========================================
        0 |  0.2   0.3   0.4   0.5   0.6   0.8
     -----------------------------------------
     0.02 | 1.24  3.58  3.30  2.18  1.49  0.72
E    0.04 | 0.82  3.43  3.55  2.41  1.29  0.56
a    0.06 | 0.40  2.92  3.78  3.03  1.87  0.66
v    0.08 |       2.10  3.91  3.74  2.51  0.87
a    0.10 |       1.20  3.88  4.27  3.16  1.21
i    0.12 |       0.64  3.33  4.71  3.67  1.60
l    0.14 |       0.35  2.27  4.73  4.21  2.07
     0.16 |             1.46  4.50  4.64  2.57
     0.20 |             1.01  3.24  4.84  3.24
     0.25 |             0.41  1.96  3.77  3.71
     0.30 |             0.22  0.95  2.45  3.62
     0.35 |             0.13  0.57  1.47  2.99
     0.40 |                   0.32  0.92  2.11
     0.50 |                   0.07  0.36  1.19
     0.60 |                         0.04  0.48
     0.80 |                               0.08
\end{verbatim}

Table II: Measured cross section per nucleon, in units 10$^{-42}$ cm$^2$ / GeV$^2$.
The row and column headers show the upper edge of the bin in $q_3$ (columns) or $E_{\mathrm{avail}}$ (rows)

\bigskip

\begin{verbatim}
                              q3
          =====================================
          |   0.2  0.3  0.4  0.5  0.6  0.8  
     ------------------------------------------
     0.02 |     0    3   10   22   36   51 
E    0.04 |     1    4   11   23   37   52 
a    0.06 |     2    5   12   24   38   53 
v    0.08 |          6   13   25   39   54 
a    0.10 |          7   14   26   40   55 
i    0.12 |          8   15   27   41   56 
l    0.14 |          9   16   28   42   57 
     0.16 |              17   29   43   58 
     0.20 |              18   30   44   59 
     0.25 |              19   31   45   60 
     0.30 |              20   32   46   61 
     0.35 |              21   33   47   62 
     0.40 |                   34   48   63 
     0.50 |                   35   49   64 
     0.60 |                        50   65 
     0.80 |                             66 
\end{verbatim}

Table III:  The 1D bin numbering scheme used for the 67 by 67 entry covariance matrix.

\clearpage
\pagebreak

\begin{verbatim}
Bin xsec
--------
 0  1.24
 1  0.82
 2  0.40
 3  3.58
 4  3.43
 5  2.92
 6  2.10
 7  1.20
 8  0.64
 9  0.35
 10 3.30
 11 3.55
 12 3.78
 13 3.91
 14 3.88
 15 3.33
 16 2.27
 17 1.46
 18 1.01
 19 0.41
 20 0.22
 21 0.13
 22 2.18
 23 2.41
 24 3.03
 25 3.74
 26 4.27
 27 4.71
 28 4.73
 29 4.50
 30 3.24
 31 1.96
 32 0.95
 33 0.57
 34 0.32
 35 0.07
 36 1.49
 37 1.29
 38 1.87
 39 2.51
 40 3.16
 41 3.67
 42 4.21
 43 4.64
 44 4.84
 45 3.77
 46 2.45
 47 1.47
 48 0.92
 49 0.36
 50 0.04
 51 0.72
 52 0.56
 53 0.66
 54 0.87
 55 1.21
 56 1.60
 57 2.07
 58 2.57
 59 3.24
 60 3.71
 61 3.62
 62 2.99
 63 2.11
 64 1.19
 65 0.48
 66 0.08
\end{verbatim}

\bigskip
Table IV:  And the cross section reordered in 67 bins which matches the
covariance matrix.

\clearpage
\pagebreak

Table V:  The data below is the upper-triangular matrix from the Cholesky decomposition U of the covariance
matrix on the cross section C, defined by C = $U^TU$. The units are
10$^{-46}$ cm$^2$ / GeV$^2$. To recover the covariance matrix, this matrix
should be premultiplied by its transpose. The first element in the first row has index (0,0).
\bigskip

{\ttfamily
%\noindent
%\begin{verbatim}
1719  643  204 3162 2758 2137 1657 1097  719  496 3459 3215 3081 2978 3149 2943 2233 1723 1143  402  236  175 1969 2346 2913 3211 3145 3416 3776 4154 3080 1648  783  557  369   81 1280 1185 1812 2386 2484 2671 3277 3540 3888 3051 1682  928  578  304   48  657  472  556  730  983 1234 1695 2036 2554 2756 2472 1643 1017  640  377   91 

   0 1064  641 3049 1208 2064 2079 1174  503  741 3307 1700  713 1692 3406 3835 2638  910  362  631  311   79 2249 1302 1120 1171 1078 1182 2675 3221 2740 1276  594  605  150   55 1347 1197  836  603  814  971  646  828 1779 2511 1647  733  762  230   29  346  675  652  680  573  569  417  402  377 1019 1880 1998 1285  623  289   39 

   0    0  439  392   24  591  644  330   76  234 1014  233   94  469 1132 1192  705   32  -94  204   92   -9  830  159   63  209  237  276  627  750  583  251  151  176   -7    3  566  418   60  -74  116  243  -90  -13  314  623  433  181  248   45    2  101  275  289  269  200  166   68    8  -39  165  497  653  432  186   62    2 

   0    0    0 4333  713 -108    1  109  210  228 2807 1367  743  541  523  677  540  354   88   40   69   36 2416 1417 1729 1723 1134  928  994  989  514  -28  -17  103   23    5 1683 1227 1468 1769 1974 1821 1813 1555  909  343 -164 -311 -204  -77    2  850  627  739  985 1272 1476 1763 1862 1771 1281  585 -202 -468 -360  -71   10 

   0    0    0    0 1975  798  313  125   26 -242 -936  271 1062 1127  534   64  -61  136  204  -93  -51    4 -834 -218   52  510 1280 1707 1241  712  326  506  251    7   68    7 -608 -430 -355 -223  162  528 1002 1384 1301  829  840  647  278  117    5 -249 -325 -300 -306 -231 -120   17  228  564  835  858  970  929  583  161   17 

   0    0    0    0    0 1452  432  134   15  -38 -440 -101  307  607  582  409  221  106  136   40   15   16 -463 -321 -297  -52  314  597  633  574  428  386  180   67   53   13 -334 -315 -457 -534 -418 -185   42  256  509  552  550  371  227   92    7 -211 -156 -203 -294 -347 -389 -410 -352 -246   68  355  576  531  335  117   13 

   0    0    0    0    0    0 1049  272  142  153   -3  -87 -254   12  458  680  566  306  184  123   58   33 -268 -156 -262 -372 -357 -254  231  573  611  272  111  115   54   19 -304 -188 -306 -478 -651 -655 -607 -475    2  397  276  135  139   66   10 -218 -116 -163 -238 -362 -471 -582 -660 -659 -403  -37  114  103   90   69   13 

   0    0    0    0    0    0    0  743  222  176   16   39 -282 -212  235  586  595  425  241  110   50   33 -258   -5  -88 -329 -376 -345  124  516  594  197   86  104   46   16 -329 -128 -126 -244 -480 -588 -601 -441    7  325  145   76   87   52   10 -182 -141 -150 -177 -274 -355 -443 -540 -488 -305  -62  -56  -50   14   47   14 

   0    0    0    0    0    0    0    0  494  205  236  237 -175 -275  -35  346  517  484  319  125   56   49   32  336  221  -74 -365 -399  -38  341  486  154   56   83   48   19  -31  116  247  240  -50 -278 -313 -249  -24   55  -52  -56   16   38    9   55   11   -6  -11  -41  -67  -76 -137 -139 -103  -81 -262 -283 -107   23   14 

   0    0    0    0    0    0    0    0    0  456 1139  383 -373 -408  107  534  547  266   78  196   99   44  802  656  406   56 -656 -851 -294  188  355   -1  -39  122   29   15  556  580  571  528  206 -142 -428 -639 -450 -140 -268 -305  -50  -11    7  257  322  287  289  236  211  151   30 -191 -258 -193 -396 -512 -301  -34    7 

   0    0    0    0    0    0    0    0    0    0 2240  683  534  285  229  112  -15 -118 -123   22   20  -14 1334  772  876  934  639  382  164   92  -63 -140  -42   11  -29   -9 1086  741  901 1130 1259 1227  982  744  425   55 -188 -162  -79  -52   -4  543  454  511  626  782  896 1030 1103 1088  828  451   98 -103 -136  -47   -2 

   0    0    0    0    0    0    0    0    0    0    0 1684  464  146  -51  -39   25   79   67   18    0    9  384  812  775  629  476  277  213   48   95   69   -1  -12    9    2  341  429  844 1070 1056  915  831  717  502  178   69   59   37   13    2  302  195  205  315  440  605  699  822  901  848  645  379  182   75   19    4 

   0    0    0    0    0    0    0    0    0    0    0    0 1557  550  232  -32  -92   -9   13  -29  -18  -11  300  153  331  633  780  913  467  250  -38   68   76   -0   -3   -7  317  189  160  330  583  720  723  843  653  194  129  119   39    7   -3  170   80  141  166  265  348  490  574  708  663  427  250  169  100   24    6 

   0    0    0    0    0    0    0    0    0    0    0    0    0 1350  311  116  -11  -40  -30  -15   -5   -9   73 -128  -11  247  410  581  382  273   25   69   58   18    4   -3   79   -4 -168 -144   38  194  253  364  345  191  152   96   42   10   -1  -12   -6   18   -3   11   16   68   94  150  187  166  168  144   82   23    4 

   0    0    0    0    0    0    0    0    0    0    0    0    0    0 1326  296  118  -50  -78   10    8  -13   20 -186 -136   -4  116  226  283  316  125   51   35   39    3   -2  -25  -52 -239 -307 -215 -103  -96  -15  157  264  149   70   48    6    0 -108  -37  -31  -58 -101 -139 -169 -190 -166  -50  100  174  138   58   18    3 

   0    0    0    0    0    0    0    0    0    0    0    0    0    0    0 1183  234   56   -4   26   15    4  -32  -44  -81 -112 -101  -45  215  369  276   68    8   40   15    5  -69  -51 -110 -188 -237 -223 -211 -140  145  307  124   46   45   15    3  -89  -52  -82 -110 -157 -200 -255 -275 -242  -26  187  172   79   28   27   10 

   0    0    0    0    0    0    0    0    0    0    0    0    0    0    0    0  896  189  144   54   17   13  -94   69    1 -123 -173 -144  121  336  362  156   49   32   19    8  -91  -55    8  -38 -172 -240 -186 -127  163  262  116   70   44   21    4  -30  -52  -98 -128 -159 -199 -243 -243 -199   17  197  121   20   12   32   13 

   0    0    0    0    0    0    0    0    0    0    0    0    0    0    0    0    0  734  277   38   14   35 -235   69   61  -43  -93  -51   29  184  314  206   91   22   41   13 -183 -122   16   36 -119 -199  -43   -2  103   96   95   85   26   34    7  -22  -91 -112 -138 -137 -155 -139 -131  -83  -29  -28  -98  -69   18   35   12 

   0    0    0    0    0    0    0    0    0    0    0    0    0    0    0    0    0    0  519   58   12   19  -98   73   53  -30  -32  -56  -67   42  246  217  121    6   15    9  -25  -81   84  111   -4  -47   68   53  110   47  100  123   49   29    3   75   -3  -32  -60  -44  -70  -61  -25   12   43   31   13   18   50   35    8 

   0    0    0    0    0    0    0    0    0    0    0    0    0    0    0    0    0    0    0  238   38   -6  179  131   19  -54 -128 -199 -171 -133   81  197  141   67   -7    3  158  162  131   90   92   -7 -124 -233 -168  -21  128  139  133   25    0   91  136  125  107   79   69   -3  -12  -88  -68   56  181  137   85   27   -1 

   0    0    0    0    0    0    0    0    0    0    0    0    0    0    0    0    0    0    0    0  130   65   49   -7  -21  -59 -159 -207 -128 -100  -15   60   46  159  120   29   34   -8  -18  -41  -90 -140  -97 -219 -264 -104  -14   61  161  110   13  -17   20  -11  -25  -39  -50  -68  -83 -171 -241 -221  -82   30  111   78    8 

   0    0    0    0    0    0    0    0    0    0    0    0    0    0    0    0    0    0    0    0    0  116 -174   30    0  -58 -172 -175  -51  -49   18   52  -13  111  133   32 -122  -99  -19  -11 -117 -179  -47 -123 -176  -60    9   43  119  112   15  -62  -67 -122 -142 -138 -125 -115 -111 -158 -160 -147  -83   13  108   84   13 

   0    0    0    0    0    0    0    0    0    0    0    0    0    0    0    0    0    0    0    0    0    0 1500  312  339  359  216   73  -54  -56  -46 -101  -29  -15  -31   -5  615  333  422  528  573  565  415  319  156  -72 -157 -106  -53  -30   -4  333  239  256  296  388  423  489  523  522  406  189  -15 -111  -92  -29   -2 

   0    0    0    0    0    0    0    0    0    0    0    0    0    0    0    0    0    0    0    0    0    0    0 1274  448  271  111  -65    4  -72   20  -38  -65  -37  -11   -1  174  275  571  688  608  486  397  298  170   15  -46  -52  -23  -10   -1  186  136  125  197  259  357  393  460  474  441  339  173   42  -11  -10   -2 

   0    0    0    0    0    0    0    0    0    0    0    0    0    0    0    0    0    0    0    0    0    0    0    0 1127  250  194  104   53  -13  -16  -27  -19  -10   -0   -1  132  163  320  412  408  365  331  285  163   11  -37  -21  -15   -3   -0  115   76   92  144  194  255  303  344  370  291  166   61   14   -4   -4   -1 

   0    0    0    0    0    0    0    0    0    0    0    0    0    0    0    0    0    0    0    0    0    0    0    0    0 1208  296  330  138   31  -67  -10   15    3   -1   -3  149  121  114  193  292  327  306  337  185  -18   -4    4    1    1   -1   87   55   91  113  157  203  272  299  326  235   87   17   12   14    1   -0 

   0    0    0    0    0    0    0    0    0    0    0    0    0    0    0    0    0    0    0    0    0    0    0    0    0    0 1327  396  174   20  -56   25   51   17    2   -2   59   36   20   79  220  301  288  355  223   40   77   93   58   20   -1   39   14   57   79  117  155  208  237  296  228  114  123  143  101   22   -1 

   0    0    0    0    0    0    0    0    0    0    0    0    0    0    0    0    0    0    0    0    0    0    0    0    0    0    0 1428  233  139  -15   47   50   20    5   -2    1    3 -110  -88   47  117  144  257  213   72   92   78   42   14   -1  -15  -28    3   -7    6   23   65   75  125  139   96   72   72   62   21    4 

   0    0    0    0    0    0    0    0    0    0    0    0    0    0    0    0    0    0    0    0    0    0    0    0    0    0    0    0 1338  288  145   65   10   14   13    2  -63  -33  -67  -86  -66  -49   18   93  236  242  120   62   27    9    2  -55  -58  -77  -93 -103 -105 -112  -97  -50  118  236  175   85   37   23   10 

   0    0    0    0    0    0    0    0    0    0    0    0    0    0    0    0    0    0    0    0    0    0    0    0    0    0    0    0    0 1371  235   58    2   13   13    2  -20  -61  -89 -124 -176 -172  -83  -15  267  306   70   22   -9   -4    2  -49  -68 -104 -140 -161 -204 -224 -217 -154   83  241  105  -18  -32   16   16 

   0    0    0    0    0    0    0    0    0    0    0    0    0    0    0    0    0    0    0    0    0    0    0    0    0    0    0    0    0    0  871  136   39   -1    1    3  -20  -68   13  -18  -90 -114  -46  -51  203  329  170  104   32    1    3  -21  -50  -90 -115 -122 -153 -200 -182 -120  113  292  229  109   40   25   13 

   0    0    0    0    0    0    0    0    0    0    0    0    0    0    0    0    0    0    0    0    0    0    0    0    0    0    0    0    0    0    0  622  139   38   24    7  -87  -57  -68  -95  -29  -81   -7  -64   12  206  311  247  133   38    5  -65  -49  -65  -87  -90  -81 -127 -111 -113    1  168  306  277  166   52    9 

   0    0    0    0    0    0    0    0    0    0    0    0    0    0    0    0    0    0    0    0    0    0    0    0    0    0    0    0    0    0    0    0  336   52   13    2   -0  -36  -98 -114  -25  -18   -5  -19   -9   59  148  172  104   30    2  -22  -18    7   -5   -6  -18  -38  -48  -33  -39  -10   94  140  112   35    4 

   0    0    0    0    0    0    0    0    0    0    0    0    0    0    0    0    0    0    0    0    0    0    0    0    0    0    0    0    0    0    0    0    0  238   60   11  -33  -15  -85 -112  -76  -94  -90  -90  -13   65   23   89  116   60    6  -64  -35  -32  -34  -57  -70  -96 -115 -112  -77   -6   46   72   84   51    9 

   0    0    0    0    0    0    0    0    0    0    0    0    0    0    0    0    0    0    0    0    0    0    0    0    0    0    0    0    0    0    0    0    0    0  153   14 -112  -71  -37  -33  -72  -93    5  -35  -12   54   15   35   46   49    7  -71  -52  -79  -80  -89  -88  -85  -77  -90  -83  -39   17   47   49   38    7 

   0    0    0    0    0    0    0    0    0    0    0    0    0    0    0    0    0    0    0    0    0    0    0    0    0    0    0    0    0    0    0    0    0    0    0   37   -7  -31   37   36   -2  -19   20  -24   -9   40   34   40   44   36    4    3   -0  -36  -38  -32  -31  -38  -22  -34   -8   44   97   84   53   31    4 

   0    0    0    0    0    0    0    0    0    0    0    0    0    0    0    0    0    0    0    0    0    0    0    0    0    0    0    0    0    0    0    0    0    0    0    0 1061  123  124  156  179  197  132   98   85  -13  -64  -29   -5   -4   -1  174  117  105   96  136  127  150  166  171  178  117   24  -40  -31   -1    3 

   0    0    0    0    0    0    0    0    0    0    0    0    0    0    0    0    0    0    0    0    0    0    0    0    0    0    0    0    0    0    0    0    0    0    0    0    0  695  179  208  230  176   98   76   -5  -52  -16  -24    5   -2   -1   84   86   94  111  128  170  184  186  164  133   89   42   -0   -6   -2   -1 

   0    0    0    0    0    0    0    0    0    0    0    0    0    0    0    0    0    0    0    0    0    0    0    0    0    0    0    0    0    0    0    0    0    0    0    0    0    0  911  377  330  274  223  157  100   30   -2   17   20    7    0   97   62   55  101  140  189  198  248  274  259  212  162   98   40    6   -2 

   0    0    0    0    0    0    0    0    0    0    0    0    0    0    0    0    0    0    0    0    0    0    0    0    0    0    0    0    0    0    0    0    0    0    0    0    0    0    0  979  271  237  198  162   93    2  -15    8   11    7   -0   77   41   42   78  114  156  178  217  243  206  138   97   62   28    3   -2 

   0    0    0    0    0    0    0    0    0    0    0    0    0    0    0    0    0    0    0    0    0    0    0    0    0    0    0    0    0    0    0    0    0    0    0    0    0    0    0    0 1054  228  180  176   63  -18   28   35   33   11   -1   52   30   47   77  112  157  183  211  226  172  101  108   99   56    7   -3 

   0    0    0    0    0    0    0    0    0    0    0    0    0    0    0    0    0    0    0    0    0    0    0    0    0    0    0    0    0    0    0    0    0    0    0    0    0    0    0    0    0 1085  185  196   88  -18   14   26   27   11   -1   51   34   51   73  104  132  162  193  215  153   68   87   95   56    7   -5 

   0    0    0    0    0    0    0    0    0    0    0    0    0    0    0    0    0    0    0    0    0    0    0    0    0    0    0    0    0    0    0    0    0    0    0    0    0    0    0    0    0    0 1131  173   84   -3    9   10   -2    3   -0   31   17   21   35   58   73  103  136  144   91   22   28   40   22    3   -2 

   0    0    0    0    0    0    0    0    0    0    0    0    0    0    0    0    0    0    0    0    0    0    0    0    0    0    0    0    0    0    0    0    0    0    0    0    0    0    0    0    0    0    0 1192  148   10    2   10    7    7   -1   26   -1    7   12   32   47   82  109  146  139   77   41   33   25    9    0 

   0    0    0    0    0    0    0    0    0    0    0    0    0    0    0    0    0    0    0    0    0    0    0    0    0    0    0    0    0    0    0    0    0    0    0    0    0    0    0    0    0    0    0    0 1085  198   32   45   22    8    0   24  -25  -47  -61  -53  -65  -64  -32   61  235  298  172   59   26   23   10 

   0    0    0    0    0    0    0    0    0    0    0    0    0    0    0    0    0    0    0    0    0    0    0    0    0    0    0    0    0    0    0    0    0    0    0    0    0    0    0    0    0    0    0    0    0  860  139   96   43    7    2  -33  -41  -66  -72  -78  -87 -129 -120  -58  137  298  261  150   61   26   10 

   0    0    0    0    0    0    0    0    0    0    0    0    0    0    0    0    0    0    0    0    0    0    0    0    0    0    0    0    0    0    0    0    0    0    0    0    0    0    0    0    0    0    0    0    0    0  614  141   81   17    2  -48  -25  -26  -29  -29   -2  -33  -30  -28   49  155  257  229  128   30    3 

   0    0    0    0    0    0    0    0    0    0    0    0    0    0    0    0    0    0    0    0    0    0    0    0    0    0    0    0    0    0    0    0    0    0    0    0    0    0    0    0    0    0    0    0    0    0    0  403  103   31    1  -10  -22  -20  -18  -11   -2  -34  -25   17   85  152  220  205  133   38    4 

   0    0    0    0    0    0    0    0    0    0    0    0    0    0    0    0    0    0    0    0    0    0    0    0    0    0    0    0    0    0    0    0    0    0    0    0    0    0    0    0    0    0    0    0    0    0    0    0  280   37    1    6    8    5    7    7   22   -0    7   28   80  128  187  167  113   35    1 

   0    0    0    0    0    0    0    0    0    0    0    0    0    0    0    0    0    0    0    0    0    0    0    0    0    0    0    0    0    0    0    0    0    0    0    0    0    0    0    0    0    0    0    0    0    0    0    0    0  122    2    5    1  -10  -11   -9   -3    5    7   22   23   23   73   83   68   32    3 

   0    0    0    0    0    0    0    0    0    0    0    0    0    0    0    0    0    0    0    0    0    0    0    0    0    0    0    0    0    0    0    0    0    0    0    0    0    0    0    0    0    0    0    0    0    0    0    0    0    0   23  -15   -6  -12  -18  -24  -29  -31  -52  -54  -49  -30  -18   -7    5   15    7 

   0    0    0    0    0    0    0    0    0    0    0    0    0    0    0    0    0    0    0    0    0    0    0    0    0    0    0    0    0    0    0    0    0    0    0    0    0    0    0    0    0    0    0    0    0    0    0    0    0    0    0  497   69   50   34   52   38   46   57   64   94   69   16  -23  -11    5    3 

   0    0    0    0    0    0    0    0    0    0    0    0    0    0    0    0    0    0    0    0    0    0    0    0    0    0    0    0    0    0    0    0    0    0    0    0    0    0    0    0    0    0    0    0    0    0    0    0    0    0    0    0  326   92   81   78   69   66   66   28   -1  -12   26   17    2    2   -3 

   0    0    0    0    0    0    0    0    0    0    0    0    0    0    0    0    0    0    0    0    0    0    0    0    0    0    0    0    0    0    0    0    0    0    0    0    0    0    0    0    0    0    0    0    0    0    0    0    0    0    0    0    0  311  107  112  116  130  112   92  -23 -109  -59   -3    8   -6   -5 

   0    0    0    0    0    0    0    0    0    0    0    0    0    0    0    0    0    0    0    0    0    0    0    0    0    0    0    0    0    0    0    0    0    0    0    0    0    0    0    0    0    0    0    0    0    0    0    0    0    0    0    0    0    0  361  108  126  134  129  113  -11  -91  -31   28   15  -12   -9 

   0    0    0    0    0    0    0    0    0    0    0    0    0    0    0    0    0    0    0    0    0    0    0    0    0    0    0    0    0    0    0    0    0    0    0    0    0    0    0    0    0    0    0    0    0    0    0    0    0    0    0    0    0    0    0  438  104  118  126  126   42  -32  -10   24   13   -9   -6 

   0    0    0    0    0    0    0    0    0    0    0    0    0    0    0    0    0    0    0    0    0    0    0    0    0    0    0    0    0    0    0    0    0    0    0    0    0    0    0    0    0    0    0    0    0    0    0    0    0    0    0    0    0    0    0    0  529  119  128  120   55   -0   22   42   21   -7   -6 

   0    0    0    0    0    0    0    0    0    0    0    0    0    0    0    0    0    0    0    0    0    0    0    0    0    0    0    0    0    0    0    0    0    0    0    0    0    0    0    0    0    0    0    0    0    0    0    0    0    0    0    0    0    0    0    0    0  621  119  116   47  -25  -15   12    9   -5   -4 

   0    0    0    0    0    0    0    0    0    0    0    0    0    0    0    0    0    0    0    0    0    0    0    0    0    0    0    0    0    0    0    0    0    0    0    0    0    0    0    0    0    0    0    0    0    0    0    0    0    0    0    0    0    0    0    0    0    0  679  121   82   29   26   29   12   -6   -5 

   0    0    0    0    0    0    0    0    0    0    0    0    0    0    0    0    0    0    0    0    0    0    0    0    0    0    0    0    0    0    0    0    0    0    0    0    0    0    0    0    0    0    0    0    0    0    0    0    0    0    0    0    0    0    0    0    0    0    0  680  145   89   40   27   17    0   -2 

   0    0    0    0    0    0    0    0    0    0    0    0    0    0    0    0    0    0    0    0    0    0    0    0    0    0    0    0    0    0    0    0    0    0    0    0    0    0    0    0    0    0    0    0    0    0    0    0    0    0    0    0    0    0    0    0    0    0    0    0  729  277  150  46   18    9    4 

   0    0    0    0    0    0    0    0    0    0    0    0    0    0    0    0    0    0    0    0    0    0    0    0    0    0    0    0    0    0    0    0    0    0    0    0    0    0    0    0    0    0    0    0    0    0    0    0    0    0    0    0    0    0    0    0    0    0    0    0    0  708  208   83   24   10    4 

   0    0    0    0    0    0    0    0    0    0    0    0    0    0    0    0    0    0    0    0    0    0    0    0    0    0    0    0    0    0    0    0    0    0    0    0    0    0    0    0    0    0    0    0    0    0    0    0    0    0    0    0    0    0    0    0    0    0    0    0    0    0  572  185   73   11   -4 

   0    0    0    0    0    0    0    0    0    0    0    0    0    0    0    0    0    0    0    0    0    0    0    0    0    0    0    0    0    0    0    0    0    0    0    0    0    0    0    0    0    0    0    0    0    0    0    0    0    0    0    0    0    0    0    0    0    0    0    0    0    0    0  416   83    8   -7 

   0    0    0    0    0    0    0    0    0    0    0    0    0    0    0    0    0    0    0    0    0    0    0    0    0    0    0    0    0    0    0    0    0    0    0    0    0    0    0    0    0    0    0    0    0    0    0    0    0    0    0    0    0    0    0    0    0    0    0    0    0    0    0    0  228   18   -1 

   0    0    0    0    0    0    0    0    0    0    0    0    0    0    0    0    0    0    0    0    0    0    0    0    0    0    0    0    0    0    0    0    0    0    0    0    0    0    0    0    0    0    0    0    0    0    0    0    0    0    0    0    0    0    0    0    0    0    0    0    0    0    0    0    0  116   12 

   0    0    0    0    0    0    0    0    0    0    0    0    0    0    0    0    0    0    0    0    0    0    0    0    0    0    0    0    0    0    0    0    0    0    0    0    0    0    0    0    0    0    0    0    0    0    0    0    0    0    0    0    0    0    0    0    0    0    0    0    0    0    0    0    0    0   34
%\end{verbatim}
}
